# Supplementary material for: Exploring the substructure of nucleons and nuclei with machine learning
Source: arXiv:2110.01924 source file (2021-10-05)
Supplement: Supplementary file 1 [file theory_appendices.tex]

%% The "\appendix" call has already been made in the declaration
%% of the "appendices" environment (see thesis.tex).

%\setsecnumdepth{subsection}
%\settocdepth{section}

%\setcounter{chapter}{-1}
%\chapter{Basics}
%\chapterquote{You first learn Newton's law of motion in terms of position and velocities of particles, then you learn about more general formulation of the equations: the Lagrangian formulation where you have quite a general dynamical coordinates, coordinates which are any functions of the position of the particles and then you have the velocities corresponding to these coordinates. Now Hamilton, a hundred years previously has setup another form of dynamics in which the coordinates are replaced by momentum variables, now you might think that this is not an important change but it led to greater symmetry and beauty in the equations, and Hamilton pursued this line of investigation just because he was thriving for mathematical beauty, I believe this shows very strongly the genius of Hamilton that he was able to follow through a line of work whose importance was not made evident until a hundred years later. I don't think there's any other such examples in the history of physics.}{Paul Dirac, From Dirac's Lectures - Christchurch, New Zealand (1975)} 
%\label{chap:0}
\chapter{Theoretical foundations}
The leap from Lagrangian~\cite{lagrange1853mecanique} and Hamiltonian~\cite{hand1998analytical} classical mechanics~\cite{landau2000mechanics,landau2013classical} to the state of the art quantum chromodynamics~\cite{cowan1964electron,
gell1964schematic,
zweig1964,
bloom1969high,
bjorken1969asymptotic,
callan1969high,
feynman1969very,
feynman2018photon,
Blumlein:2012bf,
nambu1966preludes,
faddeev1967feynman,
hooft1971renormalization,
fritzsch2002current,
fritzsch1973advantages,
gross1973ultraviolet,
politzer1973reliable}
is at the least that of the last two centuries of scientific progress. This gigantic leap is not uniform as most of the revolutionary theories and discoveries were piled rapidly within the last century, nor is it continuous as we have gained fundamentally new perspectives on nature at the scale of atoms and subatomic particles~\cite{Dirac1930-DIRTPO,peskin2018introduction}. Therefore, by no means this chapter is meant to encapsulate nor do justice this important evolution of subatomic physics; nowadays, with the level of advancements particle physics is witnessing, one might even question the relevancy of classical mechanics with respect to the main topic of this thesis. However, I think that these few pages will serve as a historical base and smooth introduction to quantum electrodynamics that I will build upon its structure and findings to introduce quantum chromodynamics and discuss my research on the hadronic structure of nucleons and nuclei. More importantly than the historical aspect and the natural connection between these theories, I will highlight in this chapter the important role symmetry played in shaping their mathematical formalisms. This specific aspect has always been a source of my fascination particularly with how it was distilled by Landau and Lifshitz in Refs.~\cite{landau2000mechanics,landau2013classical} and Dirac in Ref.~\cite{Dirac1930-DIRTPO,peskin2018introduction} which Sects.~\ref{s1:CM} and \ref{s1:CED} will be based upon.

In Sect.~\ref{s1:CM}, I discuss the theory of non-relativistic classical mechanics, that relied on an
\textit{inertial}\footnote{Inertial: a frame of reference that is not undergoing
acceleration.} reference frame with time and space as
\textit{homogeneous}\footnote{Homogeneity: various positions/instants in time and space
are equivalent.} and \textit{isotropic}\footnote{Isotropy: different orientations are
equivalent.}. This theory was adopted for centuries and was built based on the concept of absolute time and instantaneous propagation of interaction. However, it showed limitation describing light and its interaction with other particles. 

In Sect.~\ref{s1:CED}, I discuss the theory of relativistic classical mechanics in order to adress this limitation. Therefore introducing a new framework in which light has a finite speed and considered absolute (instead of time) with respect to different observers. This was rectified most generally by Einstein with his theory of special relativity~\cite{einstein2015relativity}, that reduces to Newtonian physics when the speed of the objects considered is far less than the speed of light. Building on the latter principle, Maxwell established his equations to describe light in terms of an electromagnetic field~\cite{maxwell1890scientific}. 

In Sect.~\ref{s1:QED}, I introduce quantum mechanics and electrodynamics that were a first attempt to solve the utlra-violet catastrophe~\cite{klein1961max} manifested by studying the black body radiation by means of relativistic classical mechanics. The other limitation was the photoelectric effect~\cite{einstein1905photoelectric} in which the number of emitted electrons of materials undergoing electromagnetic radiation, increased with the frequency instead of intensity (as in Maxwell's). Both of these observations required the transition from the classical point of view of seeing light as an electromagnetic wave to the quantum mechanical one where light is described as discrete bundle of energies or simply a particle.

\section{Classical mechanics} \label{s1:CM}
In classical mechanics, the state of a mechanical system is completely determined if all the coordinates and velocities are simultaneously specified. The system is characterised by a function called Lagrangian $L(\bm{q},\bm{\dot{q}},t)$ where $t$ is the absolute time and $\bm{q}$, $\bm{\dot{q}}$ are respectively the generalised coordinates and velocities of the system.

\myparagraph{Hamilton's principle of Least Action}
The motion of a mechanical system is such that the
\textit{action} defined as:
\begin{align}
    S = \int_{t_1}^{t_2} L(\bm{q},\bm{\dot{q}},t)dt,
\end{align}
takes the least possible value. Hence the motion equations are:
\begin{equation} \label{eq:Lagrange_motion_equations}
    \delta S = \int_{t_1}^{t_2} (\bm{\partial_{q}} \,L\, \cdot \bm{\delta q} + \bm{\partial_{\dot{q}}} \,L\, \cdot \bm{\delta \dot{q}}) dt =0 \implies \left(\bm{\partial_{q}} \,L\,\, - d_t \bm{\partial_{\dot{q}}} \,L\,\, \right)= 0
\end{equation}
which are invariant up to an additive total derivative to
$L$ with respect of time of some function $f(\bm{q},t)$.
%%===

\myparagraph{Galilean relativity} 
The emphasis here is on how the choice of the
relativity principle and the interpretation of space and
time dictates our laws of physics.   
Starting from the homogeneous and isotropic time and space
hypothesis, one can already make inferences concerning the
form of the Lagrangian of a particle moving freely in an
inertial frame.
 
Starting from the \textbf{Homogeneity of space and time} one deduces that
the Lagrangian cannot contain explicitly neither the radius
vector $\bm{q}$ of the particle nor the time t, i.e
$L(\bm{q},\bm{\dot{q}},t) = L(\bm{\dot{q}})$. Secondly, considering the \textbf{Isotropy of space} we further deduce that the Lagrangian must also be independent of the direction of
$\bm{\dot{q}}$, i.e $L(\bm{\dot{q}}) = L(\dot{q}^2)$. Finally and since homogeneity implies
$\bm{\partial_{\bm{q}}}\,L = 0$, we are left with
$d_t(\bm{\partial_{\bm{\dot{q}}}}\,L)=0$ from
Eq.~(\ref{eq:Lagrange_motion_equations}) hence,
$\bm{\partial_{\dot{q}}}\,L=\bm{\text{\textbf{Const}}}$ and
since it is only a function of the velocity, it follows that
$\bm{\dot{q}} = \bm{\text{\textbf{Const}}}$ which is the \textbf{Law of Inertia}.

Let us consider an inertial frame $(K)$ moving (as
of $t=0$) with velocity $\bm{\dot{\epsilon}}$ relatively to
a different frame $(K')$. The Galilean
transformations between $(K)$ and $(K')$ read:
\begin{align}
    \label{eq:galilean_transformations}
    \bm{q'} = \bm{q} + \bm{\dot{\epsilon}} t, \qquad t' &= t
\end{align} 
In order for our theory to be invariant under Eq.~(\ref{eq:galilean_transformations}), $L(\dot{q}^2)$ must then be converted by this
transformation into a function $L'$ which differs from
$L(\dot{q}^2)$, if at all, only by the total time derivative
of a function of coordinates and time. Therefore:
\begin{align}
    L' = L(\dot{q}'^2)
    = L(\dot{q}^2 + 2\bm{\dot{q} \cdot \dot{\epsilon}} + \dot{\epsilon}^2) 
    \stackrel[\text{order}]{\text{first}}{=} L(\dot{q}^2) + 2\bm{\dot{q} \cdot \dot{\epsilon}}(\partial_{\dot{q}^2}\,L)
\end{align}

Since $2\bm{\dot{q}\dot{\epsilon}}(\partial_{\dot{q}^2}\,L)$
must be a total time derivative to respect invariance, it
has to be a linear function of the velocity $\bm{\dot{q}}$,
hence $\partial_{\dot{q}^2}\,L$ should be independent of the
velocity and
therefore the Lagrangian is in this case proportional to the
square of velocity:
\begin{align}
    L &\propto \dot{q}^2 \equiv \frac{1}{2}m\dot{q}^2
\end{align}
The quantity $m$ which appears in the Lagrangian for a
freely moving particle is called the \textit{mass} of the
particle which becomes meaningful only when the additive
property is taken into account in a system of particles.

\myparagraph{System of particles interacting} 
The interaction between the particles can be described by adding to the Lagrangian, a certain function of the coordinates which depends on the nature of the interaction\footnote{This statement is only valid in classical mechanics where interactions are meant to happen instantaneously.}. We denote this function by $-U$, and thus:
\begin{align}
L = \sum_a\frac{1}{2}m_a \dot{q}_a^2 - U(\bm{q_1}, \bm{q_2},...)
\end{align}
with $q_a$, the radius vector of the $a^{th}$ particle.
We will designate the first term by a variable ${\displaystyle T =
\sum_a\frac{1}{2}m_a \dot{q}_a^2}$. $T$ and $U$ are called
respectively kinetic and potential energy and these will gain significance when we introduce formally the concept of energy.

The fact that the potential energy depends only on the
positions of the particles at a given instant shows that a
change in the position of any particle instantaneously
affects all the other particles. We may say that the
interactions are instantaneously propagated. The necessity
for interactions to be instantaneous is closely related to
the absolute nature of time in Galileo's principle of
relativity and will be invalid in relativistic mechanics.

%\myparagraph{Isotropy of time} The form of the Lagrangian: 
%\begin{align}
%    L = \sum_a\frac{1}{2}m_a \dot{q}_a^2 - U(\bm{q_1}, \bm{q_2},...)
%\end{align}
%shows that time is both homogeneous and isotropic, i.e if
%$t$ is replaced by $-t$, the Lagrangian remains unchanged
%hence if a given motion is possible in a system, so is the
%reverse motion.
%
%\myparagraph{Newton's second Law} if we substitute this
%Lagrangian, in the motion equations:
%\begin{align}
%    L = \sum_a\frac{1}{2}m_a \dot{q}_a^2 - U(\bm{q_1}, \bm{q_2},...),\,\,\, \text{in} \,\,\, d_t%(\bm{\partial_{\dot{q}_a}} L) - \bm{\partial_{q_a}} L = 0 \implies m_a d_t \bm{\dot{q}_a} = %- \bm{\partial_{q_a}} U \equiv \bm{F}
%\end{align} 
%Like $U$, $F$ depends only on the coordinates of the
%particles and not on their velocities, hence the
%acceleration depends as well only on the coordinates.

\myparagraph{Constants of motion}
During the motion of a system, there exist functions of
coordinates and velocities whose values remain constant
during the motion, and depend only on the initial
conditions. We will only consider the constants deriving from the fundamental homogeneity and isotropy of space and time, which have the important common
property of being additive.

First, and by virtue of \textbf{time
homogeneity}, the Lagrangian of a \textit{closed
system}\footnote{A closed mechanical system isn't subject to
any net force whose source is external to the system.}
system does not depend explicitly on time. The total time
derivative of the Lagrangian can therefore be written as:
\begin{align}
d_t L = \bm{\partial_{q}} L\,\bm{\dot{q}} + \bm{\partial_{\bm{\dot{q}}}}\,L\,\bm{\ddot{q}}
\end{align}
Note that if $L$ depends explicitly on time, a term
$\partial_t L$ would have to be added. Replacing
$\bm{\partial_{q}}\,L$ in accordance with Lagrange's
equations by $d_t(\bm{\partial_{\bm{\dot{q}}}}\,L)$ we
obtain:
\begin{align}
    d_t L = d_t(\bm{\partial_{\bm{\dot{q}}}}\,L)\cdot \bm{\dot{q}} + \bm{\partial_{\bm{\dot{q}}}}\,L\, \cdot \bm{\ddot{q}}
    =  \bm{\dot{u} \cdot v} + \bm{u \cdot \dot{v}}
    =  d_t(\bm{\dot{q} \cdot }\bm{\partial_{\bm{\dot{q}}}}\,L)
\end{align}
Hence we can write:
\begin{align}
    d_t(\bm{\dot{q}}\cdot \bm{\partial_{\bm{\dot{q}}}}\,L - L) \equiv d_t E = 0
\end{align}
therefore the energy $E$ is constant during the motion of a
closed system. The additivity of the energy follows
immediately from that of the Lagrangian since $E$ is a linear
function of the latter. The Lagrangian of a closed system (or one in a constant
external field) is of the form: $L = T(q,\dot{q}) - U(q)$,
where $T$ is quadratic function of the velocities.
Therefore:
\begin{align}
    \bm{\dot{q}}\cdot \bm{\partial_{\dot{q}}}\,L = 2T \implies
    E = 2T - L = 2T - T + U = T(q,\dot{q}) + U(q)
\end{align}

Second, and by virtue of
\textbf{space homogeneity}, the Lagrangian of a closed system is
unchanged by any parallel displacement of the entire system
in space. Let us therefore consider an infinitesimal
displacement $\bm{r} \rightarrow \bm{r}+\bm{\epsilon}$ and
obtain the condition for the Lagrangian to remain unchanged.
The resulting change in L:
\begin{align}
    \delta L = \sum_a \bm{\partial_{r_a}}\,L\,\cdot\delta\bm{r}_a
    =\bm{\epsilon} \cdot \sum_a \bm{\partial_{r_a}}\,L\,
    = 0 \rightarrow \sum_a \bm{\partial_{r_a}}\,L = 0
\end{align}
and since the Lagrange's equation implies:
\begin{align}
    \sum_a d_t(\bm{\partial_{\bm{\dot{q}_a}}}\,L) = d_t(\sum_a\bm{\partial_{\bm{\dot{q}_a}}}\,L) \equiv d_t(\bm{P})= 0
\end{align}
We deduce that $\bm{P} = \sum_a\bm{\partial_{\bm{\dot{q}_a}}}\,L =
\sum_a m_a\bm{\dot{q}_a}$, called the momentum of the
system, remains constant during the motion. The additivity of the momentum is evident. Moreover, unlike
the energy, the momentum of a system is equal to the sum
of its individual particles momenta $\bm{p}_a = m_a \bm{\dot{q}_a}$ whether or not their can be neglected.

%\myparagraph{Newton's third law} From the definition of
%momentum above:
%\begin{align}
%    \sum_a \bm{\partial_{q_a}}\,L = \sum_a \bm{F}_a = 0
%\end{align}
%we deduce that in a closed system, the sum of the forces on
%all the particles is zero.

\myparagraph{Canonical equations}
The Lagrangian formulation of field theory is particularly suited to relativistic dynamics because all expressions are explicitly Lorentz invariant. However we introduce in this section the Hamiltonian (or canonical) formulation that will ease our transition from classical to quantum mechanics.

While the Lagrangian formulation relies on generalised coordinates and velocities, the alternative Hamiltonian one relies on generalised coordinates and momenta:
\begin{alignat}{2}
    dL %&=  \bm{\partial_{q}}L \cdot \bm{dq} + \bm{\partial_{\dot{q}}}L \cdot \bm{d\dot{q}} \nonumber\\
       %&=  \bm{\dot{p}\cdot dq} + \bm{p \cdot d\dot{q}} \qquad && \text{Using Eq.~(\ref{eq:Lagrange_motion_equations})} \nonumber \\
       &= \bm{\dot{p}\cdot dq} + \left(d(\bm{p\cdot \dot{q}}) - \bm{\dot{q}\cdot d\dot{p}}\right) \qquad && \text{Using Eq.~(\ref{eq:Lagrange_motion_equations})} \nonumber \\
    dH & \equiv d(\bm{p\cdot \dot{q}}-L) = \bm{\dot{q}\cdot dp} - \bm{\dot{p} \cdot dq} \nonumber \\
    &H(\bm{p},\bm{q},t) = \bm{p\cdot \dot{q}} - L \qquad && \text{Hamiltonian}
\end{alignat}
Hence the Hamiltonian motion equations are:
\begin{equation}
    \label{eq:Hmotion}
    \bm{\dot{q}} = \bm{\partial_{p}}H,\qquad \bm{\dot{p}}=-\bm{\partial_{q}}H
\end{equation}

\myparagraph{Canonical transformations} 
The motion equations Eq.~(\ref{eq:Lagrange_motion_equations}) are invariant with respect to a transformation from a choice of generalised coordinates $\bm{q}$ to any other independent ones $\bm{Q}$ such as $\bm{q} \rightarrow \bm{Q} = \bm{Q}(\bm{q},t)$. Therefore the Hamiltonian equations are also invariant. One of the main advantages of the Hamiltonian formulation (that will be very relevant in Sect.~\ref{s1:QED}) is that the momenta $\bm{p}$ are independent of the coordinates $\bm{q}$ hence the transformations could be extended to:
\begin{equation}
    \bm{Q} = \bm{Q}(\bm{p},\bm{q},t), \qquad \bm{P}=\bm{P}(\bm{p},\bm{q},t)
\end{equation}
With this extension however, and in order for the Hamiltonian equations Eq.~(\ref{eq:Hmotion}) to retain their canonical form under these transformations, we must derive  conditions on $\bm{P}$ and $\bm{Q}$ which are:
\begin{equation}
    \label{eq:Canonical_conditions}
    \bm{\dot{Q}} = \bm{\partial_{P}H},\qquad \bm{\dot{P}} = - \bm{\partial_Q}H
\end{equation}
Any transformation respecting Eq.~(\ref{eq:Canonical_conditions}) is called canonical and keep the motion equations intact.

Due to the symmetry of the Hamiltonian formulation and the canonical transformations, the distinction between $\bm{Q}$ and $\bm{P}$ is irrelevant as one can see for example that setting $\bm{Q} = \bm{p}$ and $\bm{P}=-\bm{q}$ does not affect the canonical form of the equations. Taking into account this arbitrariness of nomenclature, we call $\bm{p}$ and $\bm{q}$ to be canonically conjugate quantities in the Hamiltonian formulation.

\myparagraph{Poisson brackets} 
We define the Poisson brackets to be:
\begin{equation} \label{eq:Poisson_brackets}
    \{H,f\}_{Poisson} \equiv \bm{\partial_p}H \cdot \bm{\partial_q} f - \bm{\partial_q}H \cdot \bm{\partial_p}f
\end{equation}
where $H$ is the Hamiltonian and $f=f(\bm{p},\bm{q},t)$ an arbitrary function of coordinates momenta and time and its total time derivative is:
\begin{equation}
    d_t f = \partial_t f + \{H,f\}_{Poisson}     
\end{equation}
It follows that $\{H,f\}_{Poisson}=0$ if $f$ is a constant of motion and independent of time.

The conditions relating canonically conjugate quantities in the Hamiltonian formulation can be compacted in terms of Poisson brackets that are invariant under canonical transformations:
\begin{equation} \label{eq:Canonical_conditions2}
    \{Q_i,Q_k\}_{Poisson} = 0,\qquad \{P_i,P_k\}_{Poisson} = 0, \qquad \{P_i,Q_k\}_{Poisson} = \delta_{ik}
\end{equation}
Poisson algebra appear naturally in Hamiltonian mechanics and we will see in Sect.~\ref{s1:QED} that it is only a special case of Galilean Lie algebra that satisfies Leibniz's law, that is, the bracket of commutation is also a derivation. %https://en.wikipedia.org/wiki/Poisson_algebra

%======================================== NR mechanics (end)
%======================================== 
\section{Classical electrodynamics} 
\label{s1:CED}
As shown in the previous
Sect.~\ref{s1:CM}, the interaction of
particles in non-relativistic classical mechanics is expressed by a potential
energy $U$ function of the coordinates of the interacting
particles only, hence containing the assumption of
instantaneous propagation of interactions. However, as was
evident in the late nineteenth century, this assumption
conflicted with Maxwell's equations for electromagnetism
which we will briefly summarise. the
latter, relied on light being the mediator of interaction
with a finite speed of propagation.

\myparagraph{Theory of special relativity} 
The combination of the principle of relativity with the
finiteness of the velocity of propagation of interactions leads to the theory of special relativity. One of the main consequence of this theory is that time is not absolute, and that only the
speed of light does not depend on the choice of reference
frame. That can be mathematically written as:
\begin{align}
    \label{eq:Lorentz_invariance}
    ds^2 = dt^2 - \bm{dq}^2, \qquad ds^2 = ds'^2
\end{align}
where $ds$ is the
interval in a reference frame (K)
between two infinitely close events separated by
$(\bm{dq},dt)$ and $ds'$ is the interval of the same two
events in (K').

\myparagraph{Lorentz transformations} 
As a consequence of
the interval invariance defined in
Eq.~(\ref{eq:Lorentz_invariance}), we can deduce the relativistic
transformations required to transition from an inertial
frame of reference to another, these are called the Lorentz
transformations. For an inertial frame (K) moving (as of
$t=0$) with velocity $\bm{\dot{\epsilon}}$ with respect to a
different frame (K'), they read:
\begin{align}
    \bm{q'} = \gamma(\bm{q}+\bm{\dot{\epsilon}}t), \qquad
    t' = \gamma\left(t + \bm{\dot{\epsilon}}\cdot \frac{\bm{q'}}{c^2}\right)
\end{align}
where $\gamma \equiv \left(1-\frac{\dot{\epsilon}^2}{c^2}\right)^{-\frac{1}{2}}$ is the
Lorentz factor. Note that the Lorentz transformations
reproduce the Galilean ones defined in
Eq.~(\ref{eq:galilean_transformations}) at the limit where
$\dot{\epsilon} \ll c$.

\myparagraph{Free relativistic particle} 
The simplest form the action integral could take to be
invariant under Lorentz transformations is a scalar. The
integrand must be a differential of the first order and the
only scalar of this kind is the interval $ds$ defined in
Eq.~(\ref{eq:Lorentz_invariance}). Therefore, the action of a free
particle has the form:
\begin{align}
    S = - \alpha \int_a^b ds = -\alpha \int_a^b \sqrt{c^2dt^2 - \bm{dq}^2} \equiv \int_{t_1}^{t_2} L dt =  - \alpha \int_{t_1}^{t_2} c\sqrt{1-\frac{\dot{q}^2}{c^2}}dt
\end{align}
where $\alpha$ is a positive constant characterising the
particle, $a$ and $b$ represent the events of arrival of the
particle at the initial and final position at times $t_1$
and $t_2$ and the minus sign is introduced in order that $S$
has a minimum as $\int_a^b ds > 0$.

To determine $\alpha$ we use the fact that for $c\rightarrow
\infty$ we retrieve the classical expression $L=m\dot{q}^2$.
Therefore expanding $L$ in powers of $\dot{q}/c$:
\begin{align}
    L = -\alpha \sqrt{1-\frac{\dot{q}^2}{c^2}} \stackrel{c \rightarrow \infty}{\simeq} -\alpha c + \alpha \frac{\dot{q}^2}{2c} = m\dot{q}^2
\end{align}
Since the constant $-\alpha c$ can be seen as the exact
differential $-\alpha c(d_t\,t)$, it is of no relevance in $L$
therefore we can write $L = \frac{\dot{q}^2}{2c} =
m\dot{q}^2$ and deduce that $\alpha = mc$. Therefore, the action and Lagrangian of a free particle reads:
\begin{align}
    S = -mc \int_a^b ds, \qquad L = -mc^2 \sqrt{1-\frac{\dot{q}^2}{c^2}}
\end{align}

\myparagraph{Relativistic particles interaction} 
Instead of interpreting the interaction between particles as
one particle acting on another, we can see it as one
particle creating a field around itself which in turn acts
on every other particle located in this field. In classical
mechanics, the field is only another mode of description of
the interaction but in the theory of special relativity and
due to the finite velocity of propagation of interactions
the field itself acquires physical reality. Therefore we
need to formulate our laws to describe the interaction of a
particle with a field and vice versa. 

The interaction
between a given electromagnetic field and a particle
is characterised only by the particle's
charge. The action for a \textit{charge}\footnote{Charge: a
charged particle.} in an electromagnetic field is:
\begin{align}
    \label{eq:EM_field_action}
S = S_p + S_{pf} = \int_a^b\left(-mc ds + \frac{e}{c}A^{\mu} dx_{\mu}\right)
\end{align}
where the left term is the action of a free particle, the
right term describing the electromagnetic interaction with
$e$ being the charge (in an arbitrary unit), $A^\mu = (\bm{A}, \phi/c)$ being
the four-potential of the electromagnetic field and $dx_\mu = (\bm{dq},\,dt)$, the
infinitesimal four-vector.

% Separating the spatial and time component of the potential
% field $A^\mu$ we can write Eq.~(\ref{eq:EM_field_action}) as:
% \begin{align} S = \int_{t_1}^{t_2}\left(-mc
% ds+\frac{e}{c}\bm{A} \cdot \bm{dq}-e\phi dt\right),
% \end{align} therefore: \begin{align}
% \label{eq:EMlagrangian} L =
% -mc^2\sqrt{1-\frac{\dot{q}^2}{c^2}}+\frac{e}{c}\bm{A\cdot
% \dot{q}}-e\phi. \end{align}

\myparagraph{The electromagnetic field tensor} 
The motion
equations of a charge in an electromagnetic field can be
written in four-dimensional form $F_{\mu\nu}$ called \textit{tensor field}. Starting from the
principle of least action and with some algebraic
manipulations, one gets:
\begin{alignat}{2}
    F_{\mu\nu} &= \partial_\mu A_\nu - \partial_\nu A_\mu
    \qquad &&\text{Tensor Field} \\
    F^{\mu\nu}&=-F^{\nu\mu}\qquad &&\text{Antisymmetric} \\
    F_{\mu\nu}F^{\mu\nu} &= 2\left(B^2 -
    \frac{E^2}{c^2}\right)\qquad &&\text{Invariant}\\
    \partial_{\mu}F_{\nu\eta} + &\partial_{\nu}F_{\eta\mu} +
    \partial_{\eta}F_{\mu\nu} = 0\qquad &&\text{Bianchi
    identity} \label{eq:Bianchi} 
\end{alignat}
With the above definitions and properties one can deduce the particle motion equations and expressions of the electric and magnetic field in a rather compact way:
\begin{alignat}{2}
    d_\tau p_\mu &= e F_{\mu\nu} u^\nu \qquad
    &&\text{Particle motion equations}\\ 
    E_i &= c F_{0i} = -\partial_t\bm{A} - \bm{\nabla}\phi \qquad &&\text{Electric field} \\
    B_i &= -\frac{1}{2} \epsilon_{ijk}F^{jk} = \bm{\nabla \times A} \qquad
    &&\text{Magnetic Field} 
\end{alignat}
where $\tau=\frac{1}{\gamma}dt=\frac{1}{c}ds$ is the
particle's proper time, $u^\nu$ is the four-velocity,
$A_\mu$ is the four-potential and $\epsilon_{ijk}$ is the
Levi-Civita tensor.

\myparagraph{Four-current density charge} So far, we've
considered only a punctual charge. The moment we consider
charges to be continuously distributed in space, we talk
instead of charge density $\rho$ such that:
\begin{alignat}{2}
    de &= \rho dV \qquad &&\text{Density charge}\\
    de dx_\mu &= \rho \dot{x}_\mu d^4x \equiv J_\mu d^4x = (\rho\bm{\dot{q}},c\rho)
              \qquad &&\text{Four-current density} \\
    \partial_\mu J^\mu &= 0 \qquad &&\text{Conservation} \label{eq:current_conservation}
\end{alignat}
which allows us to formulate the particle-field interaction
action in a more general way as:
\begin{equation}
    S_{pf} = \frac{e}{c} \int A^{\mu} dx_{\mu} = \frac{1}{c}\int A_uJ^\mu d^4x
\end{equation}
\myparagraph{Field motion equations}
Now that we have derived the motion equations of a particle
interacting with an electromagnetic field, We extend the
action principle to the field itself $S_f$, where for the
whole system it is:
\begin{align}
    S = S_p + S_{pf} + S_f = -mc\int ds + \frac{1}{c}\int A_uJ^\mu d^4x - \frac{1}{4\mu_0c}\int F_{\mu\nu}F^{\mu\nu}d^4x
\end{align}

\myparagraph{Maxwell's equations} To derive Maxwell's
equations that describes the motion of the electromagnetic
field, it suffices to (1) derive the principle of least
action on $S_{pf} + S_f$ with respect to $A_\mu$ and (2)
consider the electromagnetic tensor's Bianchi idendity
Eq.~(\ref{eq:Bianchi}) which leads to:
\begin{alignat}{2}
    (1)\quad \delta S &= \frac{1}{\mu_0c}\int(\partial_\mu
    F^{\mu\nu} + \mu_0 J^\nu)\delta A_\nu d^4x = 0 \\
    &\implies \partial_\mu F^{\mu\nu} = -\mu_0 J^\nu 
    \begin{cases} 
        \bm{\nabla\cdot E} &= \frac{\rho}{\epsilon_0} \quad
        \text{Gauss}\\
        \bm{\nabla \times B} - \frac{1}{c^2}\partial_t\bm{E}
    &= \mu_0\bm{J} \quad \text{Amp\'{e}re} \end{cases} \\
    \nonumber \\
    (2)\quad \partial_{\mu}&F_{\nu\eta} +
    \partial_{\nu}F_{\eta\mu} + \partial_{\eta}F_{\mu\nu} =
    0 \\
    &\implies
    \begin{cases} 
        \bm{\nabla\cdot B} &= 0 \quad \text{Gauss}\\
        \partial_t\bm{B} + \bm{\nabla \times E} &= \bm{0}
        \quad \text{Maxwell-Faraday}
    \end{cases}
\end{alignat}

\myparagraph{Gauge invariance} The Lagrangian is defined only up to an additive total time derivative of any function of coordinates and time:
\begin{equation}
L \rightarrow L' = L + d_t f(\bm{q},t) \implies \delta S = \delta S'    
\end{equation}
The reason being that this quantity does not contribute to the Action variation. This redundant degree of freedom is called \textit{gauge} freedom. The transition from $L$ to $L'$ is called gauge transformation. Gauge fixing or choosing a gauge denotes a specific choice of this degree of freedom which can be useful to simplify some calculations while describing the same physics.

Similarly, in electrodynamics, since $F_{\mu\nu} = \partial_\mu A_\nu - \partial_\nu A_\mu$, we have the following gauge transformation:
\begin{align}
    A^\mu \rightarrow \tilde{A}^\mu = A^\mu + \partial^\mu \chi \implies \delta S = \delta \tilde{S} \implies
    \begin{cases} 
        \bm{E} = \bm{\tilde{E}} = -\partial_t\bm{A} - \bm{\nabla}\phi \\
        \bm{B} = \bm{\tilde{B}} = \bm{\nabla \times A} 
    \end{cases}
\end{align}
Two of the most used gauge fixings in electrodynamics are:
\begin{enumerate}
    \item Coulomb gauge: $\bm{\nabla}\cdot \bm{A}(\bm{q},t) = 0$ which leads to simple wave equations when no sources are present and simple for far field radiation problems.
    \item Lorenz gauge: $\partial_\mu A^\mu = 0$ which is Lorentz invariant, and commonly used because it leads to similar wave equations for both $\phi$ and $\bm{A}$.
\end{enumerate}
In the next section, we will also emphasize on the importance of gauge fixing in quantum electrodynamics.
%======================================== R mechanics (end)
%======================================== 
\section{Quantum electrodynamics} \label{s1:QED}

%\subsection{QED Lagrangian}
%\label{s2:QED_Lagrangian}
% read https://www.quantamagazine.org/what-is-a-particle-20201112/ and shape the intro of this chapter.
% Define operators in quantum mechanics, Read "Single particle systems" in https://en.wikipedia.org/wiki/Canonical_quantisation#First_quantisation 
% first and second quantisation, why do we quantize a field? (https://en.wikipedia.org/wiki/quantisation_of_the_electromagnetic_field)
% transition through poisson brackets http://www.phys.lsu.edu/~jarrell/COURSES/ADV_SOLID_HTML/Other_online_texts/Fradkin/webusers.physics.illinois.edu/~efradkin/phys582/582-chapter4.pdf 
% Canonical quantisation of EM: https://www.damtp.cam.ac.uk/user/tong/qft/six.pdf

Classical electrodynamics summarized in the previous section, fails to describe \textit{elementary}\footnote{Elementary: on the atomic and subatomic scale.} particles and their interactions.
So far, we have only considered particles in the classical view of mechanics as point-like mathematical constructs behaving like macro-scale objects we see with naked eyes. This view is altered completely when describing particles at the \textit{quantum-scale}\footnote{quantum-scale: typically the size of atoms and lower, around $\simeq 100$ pm.}. The first failures of classical electrodynamics were observed with the black body radiation spectrum~\cite{klein1961max} and photoelectric effect~\cite{einstein1905photoelectric}.

Non-relativistic quantum mechanics was proposed as a quantized particle theory in which electromagnetic waves are seen as discrete quanta of energy (photons) and particles described as collapsed probability wave functions~\cite{Dirac1930-DIRTPO}. However, quantum mechanics was not consistent with the principle of special relativity and failed to describe the dynamics of particles moving with a velocity close to the speed of light. The remedy was achieved with the quantum electrodynamics theory, in which fields (instead of particles) are quantized and could only oscillate in discrete amounts, an idea that was extrapolated not only to photons but also to all the other elementary particles which became merely excitations of quantum fields that fill all of space~\cite{peskin2018introduction}.

The transition from a classical to quantum theory requires methods of quantisation such as the canonical~\cite{Dirac1930-DIRTPO, hall2013quantum} or the path integral~\cite{weinberg1995quantum}.
The canonical quantisation is a procedure introduced by Paul Dirac based on the classical canonical conditions in the Hamiltonian formulation introduced in Eq.~\ref{eq:Canonical_conditions2}. In the following, we will revisit very briefly quantum mechanics to deduce the correspondence principle which is at the origin of canonical quantisation, and then use it directly in the context of quantum field theory, where fields are to be quantized instead of being treated as wave-functions as in quantum mechanics.

%We further introduce elements of group theory, namely the Galilean (Sect.~\ref{s2:Galilean_group}) and the Lorentz (Sect.~\ref{s2:Lorentz_group}) groups in order to obtain a precise distinction between the relativistic properties of elementary quantum mechanical systems and those which are also shared by non-relativistic systems.

\myparagraph{Non-relativistic quantum mechanics} In the context of quantum mechanics, a particle is represented by a \textit{wave function}\footnote{Wave function: probability amplitude of finding a particle in a certain position or carrying a certain momentum.} that is a superposition of states Eq.~(\ref{eq:Superposition_of_states}). The act of measuring the state of a particle Eq.~(\ref{eq:Measuring_state_energy}) collapses its wave function. The evolution of the particle state in time is dictated by Shr\"{o}dinger equation Eq.~(\ref{eq:Shrodinger_equation}) in which the operators are non-dependent on time or equivalently by the Heisenberg equation Eq.~(\ref{eq:Heisenberg_equation}) in which the operators incorporate time dependency while the wave function does not. The free particle solution of the Shr\"{o}dinger equation is given by Eq.~(\ref{eq:free_particle_QM}). The probability amplitude for a particle to travel from one point $(\bm{x_1},t_1)$ to a later different point $(\bm{x_2},t_2)$, i.e the propagator is given by Eq.~(\ref{eq:QM_propagator}).
%more info here: https://web2.ph.utexas.edu/~vadim/Classes/2019f/brackets.pdf
\begin{alignat}{2}
    \ket{\psi} &= \sum_n a_n \ket{\psi_n} \qquad && \text{Superposition of states} \label{eq:Superposition_of_states}\\
    \hat{H} \ket{\psi_n} &= E_n \ket{\psi_n} \qquad && \text{Measuring a state's energy}
    \label{eq:Measuring_state_energy} \\ 
    i\hbar (\partial_t &+ \frac{\hbar^2}{2m} \bm{\nabla}^2_x)\psi = 0 \qquad && \text{Shr\"{o}dinger equation}
    \label{eq:Shrodinger_equation} \\ 
    d_t \hat{A}(t) &= -\frac{i}{\hbar}[\hat{A},\hat{H}]+\partial_t \hat{A}\qquad && \text{Heisenberg equation}
    \label{eq:Heisenberg_equation} \\ 
    \psi(\bm{x},t) &\propto e^{i(\bm{p}\cdot{r}-Et)/\hbar} \qquad && \text{Free particle solution} \label{eq:free_particle_QM} \\
    G(\bm{x_2},t_2,\bm{x_1},t_1) &\propto e^{-\frac{m(\bm{x_2}-\bm{x_1})^2}{2i\hbar(t_2-t_1)}} \qquad && \text{Free particle propagator} \label{eq:QM_propagator} 
\end{alignat}

By comparing Eq.~(\ref{eq:Heisenberg_equation}) to the classical Poison brackets Eq.~(\ref{eq:Poisson_brackets}) Paul Dirac and by virtue of the \textit{correspondence principle}\footnote{Correspondence principle: quantum equations of states must reduce to their classical form in the limit $\hbar \rightarrow 0$.} connected the two as in Eq.~(\ref{eq:Correspondence_principle}) and introduced the canonical quantisation, \textit{i.e} replacing any classical variable $A$ by its quantum counter part $\hat{A}$ as follows:
\begin{alignat}{2}
    & \begin{cases} %see https://physics.stackexchange.com/questions/19770/what-is-the-connection-between-poisson-brackets-and-commutators
    \{A,H\}_{Poisson} &\rightarrow -\frac{i}{\hbar} [\hat{A},\hat{H}] \\
    H&\rightarrow \hat{H} = i\hbar \partial_t\\
    p&\rightarrow \hat{p} = -i\hbar\bm{\nabla_x}\\
    x&\rightarrow \hat{x} = x
    \end{cases}&& \text{Correspondence principle} \label{eq:Correspondence_principle} 
\end{alignat}
Any operator can be expressed in either one of the canonical variables spaces: position $\bm{x}$, Eq.~(\ref{eq:Position_space}) or momentum $\bm{p}$, Eq.~(\ref{eq:Momentum_space}). This duality stems from the Heisenberg uncertainty principle Eq.~(\ref{eq:Heisenberg_uncertainty}) translating the fact that position and momentum cannot be simultaneously known to arbitrary precision and the de Broglie relation $p=\frac{h}{\lambda}$ stating that a momentum $p$ of a particle is anti-proportional to it's wavelength $\lambda$ translating the particle-wave duality. 
\begin{alignat}{2}
    \braket{[\hat{x},\hat{p}]} &= i\hbar \qquad && \text{Canonical commutation relation} \label{eq:Canonical_commutation_relation}\\
    \Delta_x \Delta_p &\geq \frac{1}{2i}\braket{[\hat{x},\hat{p}]} = \frac{\hbar}{2} \qquad && \text{Heisenberg uncertainty principle} \label{eq:Heisenberg_uncertainty}\\
    & \begin{cases} 
        \bm{\hat{x}} \ket{\psi_n(\bm{x})} &= \bm{x_n}\ket{\psi_n(\bm{x})}\\
        \bm{\hat{p}} \ket{\psi_n(\bm{x})} &= -i\hbar \bm{\nabla_x} \ket{\psi_n(\bm{x})}
    \end{cases} \qquad && \text{Position space} \label{eq:Position_space}
    \\ & \begin{cases} 
        \bm{\hat{x}} \ket{\psi_n(\bm{p})} &= i\hbar \bm{\nabla_p} \ket{\psi_n(\bm{\bm{p}})}\\
        \bm{\hat{p}} \ket{\psi_n(\bm{p})} &= \bm{p_n} \ket{\psi_n(\bm{p})}
    \end{cases} \qquad && \text{Momentum space} \label{eq:Momentum_space}
\end{alignat}
The Galilean invariance of the Shr\"{o}dinger equation Eq.~(\ref{eq:Shrodinger_equation}) is usually overlooked, and we will briefly discuss how it describes spinless particles with mass $m$ in non relativistic quantum mechanics~\cite{LevyLeblond:1967zz}. 
Let us consider $\psi_n(\bm{p})$ a state $n\in[-s,\dddot{},\,+s]$ expressed in momentum space, then by applying the Galilean transformation $\mathcal{U}(\bm{R},\bm{\dot{\epsilon},\bm{a},b})$ defined in Appendix.~(\ref{s2:Galilean_group}) we get:
\begin{equation}
\psi_n'(\bm{p}) = \mathcal{U}\, \psi_n(\bm{p}) = e^{(iEb - i\bm{p\cdot a})} \sum_{m=-s}^{+s} D^s_{nm}(\bm{R}) \psi_m(\bm{R}^{-1}(\bm{p}-m\bm{\dot{\epsilon}}))  \label{eq:NR_wavefunction_representation}
\end{equation}
where $E=\frac{\bm{p}^2}{2m}$ and $D^s$ is the $(2s+1)$-dimensional unitary\footnote{Unitary: as it satisfies ${\displaystyle |\psi|^2 = \sum_{n=-s}^{+s} \int d^3p|\psi_n(\bm{p})|^2 = 1}$.} representation of the rotation group and $\psi_n(\bm{p})$ is the wave function of a particle with mass $m$ and spin $s$.

Galilean invariance requires that a transformed $\psi'$ differs only by a phase factor:
\begin{align} 
\text{Galilean invariance} &\implies \psi(\bm{x'},t') = e^{if(\bm{x},t)} \psi(\bm{x},t) \label{eq:Galilean_Invariance_SE}\\
\text{Shr\"{o}dinger equation}& \implies f(\bm{x},t)=\frac{1}{2}m \bm{\dot{\epsilon}}^2t + m\bm{\dot{\epsilon}}\cdot \bm{R}\cdot\bm{x} \label{eq:Shrodinger_condition}
\end{align} 
Thus by comparing Eq.~(\ref{eq:Galilean_Invariance_SE}, \ref{eq:Shrodinger_condition}) to the general non relativistic particle representation Eq.~(\ref{eq:NR_wavefunction_representation}) we conclude that the Shr\"{o}dinger equation must describe a spinless particle ($s=0$) with mass $m$.

\textbf{Important note:} It is common to work with Planck units in quantum electrodynamics so for the rest of the thesis we will use $c=1$, $\hbar = \frac{h}{2\pi} = 1$, $\epsilon_0=1$ and $\mu_0=\frac{1}{\epsilon_0 c^2}=1$, the speed of light, reduced Planck constant, permittivity and permeability respectively in Planck units. Implying that, $[length]=[time]=[energy]^{-1}=[mass]^{-1}$.

\myparagraph{Canonical quantisation of the electromagnetic field} 
%see http://www.damtp.cam.ac.uk/user/tong/qft/six.pdf 
%See section 5.2 of Lie algebra book
Quantum mechanics describes particles as wave functions that are bounded by probability conservation, hence fails to describe the creation and annihilation of particles allowed by $E=mc^2$. For that reason, and among others, we head towards a quantum field theory in which the field can be visualized as three-dimensional harmonic oscillators that oscillate with discrete energies. In this schematic picture, every excitation of the field is seen as a particle.

The quantization procedure of the electromagnetic field is complicated by the gauge invariance which renders one of degrees of freedom unphysical. We choose to work in the Lorentz gauge wherein the free theory is:
\begin{alignat}{2}
    L_f &= -\frac{1}{4} F_{\mu\nu}F^{\mu\nu} %- \frac{1}{2}(\partial_\mu A^\mu)^2
    \qquad &&\text{Field Lagrangian} \\
    F_{\mu\nu} &= \partial_\mu A_\nu - \partial_\nu A_\mu \qquad && \text{Tensor field} \\
    \partial_\mu F^{\mu\nu} + \partial^\nu(\partial_\mu A^\mu)&=\partial_\mu \partial^\mu A^\nu= 0 \qquad && \text{Field motion equations}
\end{alignat}
According to the canonical conditions Eq.~(\ref{eq:Canonical_conditions2}) and the canonical commutation relation Eq.~(\ref{eq:Canonical_commutation_relation}), the field $A_\mu$ and its conjugate momentum $\pi^\mu = \frac{\partial L}{\partial \dot{A}_\mu}$ obeys:
\begin{align}
    [A_\mu(\bm{x}),A_\nu(\bm{y})] &= [\pi^\mu(\bm{x}),\pi^\nu(\bm{y})] = 0 \\
    [A_\mu(\bm{x}),\pi_\nu(\bm{y})] & = i g_{\mu\nu}\delta^{(3)}(\bm{x}-\bm{y})
\end{align}
However, for convenience, we choose to work with another set of conjugate operators, the annihilation $a$ and creation operators $a^\dagger$ that are derived from the quantisation of the harmonic oscillator (HO) to the free scalar field. This is motivated by the fact that the quantum HO is one of the few quantum-mechanical systems for which an exact analytical solution is known~\cite{griffiths2018introduction}. The canonical transformation between $A_\mu$ and $\pi^\mu$ to $a$ and $a^\dagger$ is translated by the following \textit{Fourier transform}\footnote{Fourier transform: decomposes functions depending on momentum to functions depending on space and vice versa as in: $\phi(\bm{x},t) = \int \frac{d^3p}{(2\pi)^3} e^{i\bm{p}\cdot \bm{x}}\phi(\bm{p},t)$.}:
\begin{align}
    A_\mu(\bm{x}) &= \int \frac{d^3p}{(2\pi)^3}\frac{1}{\sqrt{2|\bm{p}|}} \sum^3_{\lambda=0}\left[a_{\bm{p}}^\lambda \epsilon_\mu^\lambda e^{i\bm{p}\cdot \bm{x}} + a_{\bm{p}}^{\lambda\,\dagger} \epsilon_\mu^{*\lambda} e^{-i\bm{p}\cdot \bm{x}} \right] \\
    \pi^\mu(\bm{x}) &= i\int \frac{d^3p}{(2\pi)^3} \sqrt{\frac{|\bm{p}|}{2}}\sum_{\lambda=0}^3\left[a_{\bm{p}}^\lambda (\epsilon^\mu)^\lambda e^{i\bm{p}\cdot \bm{x}} - a_{\bm{p}}^{\lambda\,\dagger} (\epsilon^{*\mu})^\lambda e^{-i\bm{p}\cdot \bm{x}} \right]
\end{align} 
where $\epsilon^\lambda_\mu(p)$ is a basis of polarization vectors depending on the photon four-momentum. Due to Lorentz gauge $\partial_\mu A^\mu=0$, $\epsilon^\lambda_\mu$ are transversal and obey $p^\nu\epsilon^\lambda_\nu = p^\nu \epsilon^{*\lambda}_\nu =0$. $\eta^{\lambda \lambda'}$ is the polarisation metric and is usually chosen to be aligned with the photon propagation direction $\bm{p}=(0,0,p_z)$.% and the time direction then $\epsilon^0_\mu(\bm{p})=(1,0,0,0)$ and $\epsilon^3_\mu = (0,0,0,1)$. 
Based on the properties we know about the quantisation of the harmonic oscillator~\cite{griffiths2018introduction}, we can now write the Hamiltonian of a free scalar field theory of light as follows:
\begin{gather}
    H = \int \frac{d^3p}{(2\pi)^3}E_{\bm{p}}\sum_{\lambda=1,2}a^{\lambda,\dagger}_{\bm{p}}a^\lambda_{\bm{p}} \\
    [a^{\lambda}_{\bm{p}},a^{\lambda'}_{\bm{q}}] = [a^{\lambda}_{\bm{p}},a_{\bm{p}}^{\lambda'\,\dagger}] =0,\quad \text{and} \quad [a^{\lambda}_{\bm{p}},a_{\bm{q}}^{\lambda'\,\dagger}] = -\eta^{\lambda \lambda'} (2\pi)^3 \delta^{(3)}(\bm{p}-\bm{q}) \label{eq:bose-einstein} \\
    a^\lambda_{\bm{p}}\ket{0} = 0,\quad \text{and} \quad \ket{\bm{p,\lambda}} \equiv a^{\lambda \dagger}_{\bm{p}}\ket{0} %= \sqrt{2E_{\bm{p}}}a^{\lambda \dagger}_{\bm{p}}\ket{0}
\end{gather} %https://www.imperial.ac.uk/media/imperial-college/research-centres-and-groups/theoretical-physics/msc/current/qed/Photons.pdf

We finally, summarized the quantisation of the electromagnetic field using the canonical commutation relations. A direct implication of this derivation is that annihilation/creation operators obey the Bose-Einstein statistics in which swaping two boson leave the state of the system unchanged, and that can be easily seen in Eq.~(\ref{eq:bose-einstein}).

\myparagraph{Coupling to matter} The first attempt to build a quantized relativistic free particle theory started by considering the relativistic energy-momentum relationship:
\begin{equation} \label{eq:energy-momentum}
    p_\mu p^\mu = E^2 - |\bm{p}|^2 = m^2
\end{equation}
then by canonical quantisation using Eq.~(\ref{eq:Correspondence_principle}) one gets the Klein-Gordon equation:
\begin{equation}
    \left(\bm{\nabla}^2 -\partial^2_{t^2} \right) \psi(\bm{x},t) = m^2 \psi(\bm{x},t)
\end{equation}
which leads to the plane waves particle solution: $\psi(\bm{x},t) \propto e^{-p_\mu x^\mu}$ with the problem of negative energy solutions $E=\pm\sqrt{p^2+m^2}$  associated with negative probabilities.

Dirac searched for an alternative equation in which time and space derivatives are of the first order while still being Lorentz invariant, therefore considered instead the square root form of Eq.~(\ref{eq:energy-momentum}):
\begin{equation}
    E = \sqrt{|\bm{p}|^2+m^2}
\end{equation}
and made the following analogy with the Klein-Gordon equation:
\begin{alignat}{2}
    &\left(\bm{\nabla}^2 - \partial^2_{t^2} \right) = -\beta^2( \bm{\alpha} \cdot \bm{\nabla} + \partial_t)^2 \qquad && \text{Analogy} \label{eq:KG-analogy}\\
    &\implies \begin{cases} 
        \{\alpha_i,\alpha_j\} &= \delta_{ij} \\
        \{\alpha_i, \beta\} &= 0 \quad \forall i \\
        \beta^2 &= 1
    \end{cases} \qquad && \text{Conditions} \label{eq:Dirac-conditions}\\
    & \left(\beta m + \bm{\alpha}\cdot \bm{\nabla}\right)\psi(\bm{x},t) = i\partial_t \psi(\bm{x},t) \qquad && \text{Dirac equation} \label{eq:QMv0-Dirac-equation}
\end{alignat}
the equation has to satisfy the conditions Eq.~(\ref{eq:Dirac-conditions}) in order to reproduce Klein-Gordon when squared. It is found that all representations of such algebra Eq.~(\ref{eq:Dirac-conditions}) can be obtained from those of a Clifford algebra (see Appendix.~(\ref{s2:Lorentz_group})) with dimension 4:
\begin{equation}
    \{\gamma_i,\gamma_j\} = \begin{cases} 2 \delta_{ij} \quad &\text{Galilean group} \\ 2 g_{ij} \quad &\text{Lorentz group} \end{cases} \quad \iff \quad \begin{cases} \gamma^0\alpha_i=\gamma^i \\ \beta = \gamma^0 \end{cases}  
\end{equation}
Therefore, this condition is met if and only if $\alpha_i$ and $\beta$ are $(4\times4)$ matrices following Clifford algebra which implies that the wave function has four components.
We therefore deduce that the Dirac equation explains naturally the appearance of two-component wave functions in Pauli's theory of spin~\cite{pauli1925zusammenhang}.

Substituting $\bm{\alpha}$ and $\beta$ by the $\gamma^\mu$ matrices in Eq.~(\ref{eq:QMv0-Dirac-equation}), the Dirac equation could finally be written as:
\begin{gather}\label{eq:QMv1-Dirac-equation}
i \gamma^\mu \partial_\mu \psi - m\psi = 0 \\
\text{with: }\gamma ^{0}={\begin{pmatrix}\bm{I_2}&0\\0&-\bm{I_2}\end{pmatrix}}~,\gamma ^{i}=\left({\begin{array}{cccc}0&\bm{\sigma_{i}}\\-\bm{\sigma_{i}}&0\end{array}}\right)
\end{gather}
where $\sigma_{x,y,z}$ are the $(2\times 2)$ are the spin-$1/2$ representation of SU(2) algebra, i.e Pauli matrices (see Appendix.~\ref{s3:SU2}) and $I_i$ the identity matrix of dimension $i$ and where the boost and rotation generators are given by Eq.~(\ref{eq:Clifford_algebra}).

The Dirac equation leads to a solution of the form:
\begin{equation} \label{eq:Dirac_field_solution}
    \psi(x^\mu) = u(p^\mu)e^{-p_\mu x^\mu},
\end{equation}
a product of a plane wave and a Dirac spinor $u(p^\mu)$ which can be obtained from the motion equation of the Lagrangian:
\begin{equation}
 L_{Dirac} = \bar{\psi}(i\gamma^\mu \partial_\mu - m)\psi
\end{equation}
%Fermi-stat https://www.damtp.cam.ac.uk/user/tong/qft/five.pdf
where $\bar{\psi} \equiv \psi^\dagger \gamma^0$ chosen to make the latter Lorentz invariant with $\psi^\dagger = (\psi^*)^T$ the complex conjugate of $\psi$ transposed. This solution, once quantized, will describe the behavior of spin-$1/2$ particles or simply fermions. By plugging the solution back into the Dirac equation Eq.~(\ref{eq:QMv1-Dirac-equation}) for a particle (with $p^\mu \neq 0$) we get:
\begin{equation}
    (\gamma^\mu p_\mu - m) (u_A\,\,u_B) = {\begin{pmatrix} (E-m)\bm{I_2} & -\bm{\sigma \cdot p} \\ \bm{\sigma \cdot p} & -(E-m)\bm{I_2}  \end{pmatrix}} {\begin{pmatrix} u_A \\ u_B \end{pmatrix}}=0
\end{equation}
where $u_{A,B}$ are the $(1\times 2)$ upper and lower components of $u$ respectively. Therefore:
\begin{equation}
u_A = \frac{\bm{\sigma \cdot p}}{(E-m)\bm{I_2} }u_B \qquad u_B=\frac{\bm{\sigma \cdot p}}{(E+m)\bm{I_2} }u_A
\end{equation}
The four solutions are obtained by setting successively $u_A$ and $u_B$ to the two different spin states, up: $\begin{pmatrix} 1 \\ 0 \end{pmatrix}$ and down: $\begin{pmatrix} 0 \\ 1 \end{pmatrix}$ as follows:
%http://physics.gu.se/~tfkhj/TOPO/DiracEquation.pdf
\begin{align}
u^1&=\left(1,\quad 0,\quad p_z/(E+m),\quad (p_x+ip_y)/(E+m)\right) \nonumber\\
u^2&=\left( 0,\quad  1,\quad  (p_x-ip_y)/(E+m),\quad  -p_z/(E+m)\right) \nonumber\\
u^3&=\left(-p_z/(-E+m),\quad (-p_x-ip_y)/(-E+m),\quad 1,\quad 0\right) \nonumber\\
u^4&=\left((-p_x+ip_y)/(-E+m),\quad p_z/(-E+m),\quad 0,\quad 1\right) \label{eq:Dirac_solutions}
\end{align}
For a fermion and anti-fermion with momentum $\bm{p}$ along the $z$-axis:
\begin{itemize}
    \item $u^1$ and $u^2$ describe the spin-up and spin-down fermion of energy $E=+\sqrt{m^2 + \bm{p}^2}$ and momentum $\bm{p}$
    \item $u^3$ and $u^4$ the spin-up and spin-down with energy $E=-\sqrt{m^2 + \bm{p}^2}$ and momentum $\bm{p}$. We will define $v^1=u^4(-p)$ and $v^2=u^3(-p)$ instead to translate the fact that they're positive energy anti-fermion states.
\end{itemize}
Both positive and negative energy states solutions in Dirac equations were interpreted to be associated with positive probabilities and therefore not problematic. Dirac attributed the negative energy solutions to positive energy \textit{antiparticle}~\cite{dirac1928quantum,dirac1930theory} propagating forward in time. The prediction of antiparticles was one of the main features of Dirac's theory that was later confirmed by the discovery of positrons~\cite{anderson1933positive}. %(see https://alpha.physics.uoi.gr/foudas_public/APP/Lecture5-Klein-Gordon-Dirac.pdf)

We can now write the general solution of the Dirac equation as a superposition of the solutions given in Eq.~(\ref{eq:Dirac_field_solution}):
\begin{align}
    \psi(x)&=\int \frac{d^3p}{(2\pi)^3}\frac{1}{\sqrt{2E_p}}\sum_s\left(a^s_{\bm{p}}u^s(\bm{p})e^{-ip^\mu x_\mu}+ b^{s\dagger}_{\bm{p}}v^s(\bm{p})e^{ip^\mu x_\mu}\right)\\
    \bar{\psi}(x)&=\int \frac{d^3p}{(2\pi)^3}\frac{1}{\sqrt{2E_p}}\sum_s\left(b^s_{\bm{p}}\bar{v}^s(\bm{p})e^{-ip^\mu x_\mu}+ a^{s\dagger}_{\bm{p}}\bar{u}^s(\bm{p})e^{ip^\mu x_\mu}\right)
\end{align}
where $\sum_s$ is the sum over all the spin-states and $a^s_{\bm{p}}$, $b^s_{\bm{p}}$ are simply the Fourier-coefficients so far.
%A more general definition, is the helicity $h$ where we project spin along %the particle's momentum direction:
%\begin{equation}
%    h=\frac{\bm{S \cdot p}}{|\bm{S}||\bm{p}|} = \begin{cases} +1 &\quad \text%{right-handed} \\ -1 &\quad \text{left-handed} \end{cases}
%\end{equation}

In order to canonically quantize the Dirac field, $\psi$ and the Fourier-coefficients are promoted as quantum operators where $a^s_{\bm{p}}$ corresponds to the annihilation operator (for a fermion), $b^s_{\bm{p}}$ (for an anti-fermion) and $a^{s\dagger}_{\bm{p}}$ the creation operator (for a fermion), $b^{s\dagger}_{\bm{p}}$ (for an anti-fermion).
In the case of the electromagnetic field quantisation, the commutation relations of the creation/annihilation operators, specifically Eq.~(\ref{eq:bose-einstein}), dictated completely that the photons follow Bose-Einstein statistics. Fermions however are spin-$1/2$ particles that obey Fermi-Dirac statistics with the quantum state picking up a minus sign upon the interchange of any two particles. This fact is embedded into the structure of relativistic quantum field theory where a particle is represented by the Lorentz group who's algebra (App.~\ref{s2:Lorentz_group}) is dictated by the anti-commutation relations: %https://www.damtp.cam.ac.uk/user/tong/qft/five.pdf
\begin{equation}
    \{a^{r}_{\bm{p}},a^{s\dagger}_{\bm{q}}\} = \{b^{r}_{\bm{p}},b^{s\dagger}_{\bm{q}}\} = (2\pi)^3\delta^{(3)}(\bm{p}-\bm{q})\delta^{rs} \\
    \{a^{r}_{\bm{p}},a^{s}_{\bm{q}}\} = \{a^{r\dagger}_{\bm{p}},a^{s\dagger}_{\bm{q}}\} = \{b^{r}_{\bm{p}},b^{s}_{\bm{q}}\} = \{b^{r\dagger}_{\bm{p}},b^{s\dagger}_{\bm{q}}\} = 0
    \end{equation}
which therefore implies:
\begin{align}
    \{\psi_\alpha(\bm{x}),\psi_\beta(\bm{y})\} &= \{\psi^\dagger_\alpha(\bm{x}),\psi^\dagger_\beta(\bm{y})\} = 0 \\
    \{\psi_\alpha(\bm{x}),\psi^\dagger_\beta(\bm{y})\} &= \delta_{\alpha \beta}\delta^{(3)}(\bm{x}-\bm{y})
\end{align}
%https://www.desy.de/~jlouis/Vorlesungen/QFTI10/QFTI.pdf
Finally we can write the full quantum electrodynamic Lagrangian using the quantised electromagnetic and Dirac fields as well as their interaction term as:
\begin{align}   \label{eq:L_QED}
    L_{QED} &= L_{Maxwell} + L_{Dirac} + L_{int}\\
            &= -\frac{1}{4} F_{\mu\nu}F^{\mu\nu} + \sum_{j} \bar{\psi}_j(i\gamma^\mu \partial_\mu - m_j)\psi_j - \overbrace{\sum_{j} q_j \bar{\psi}_j\gamma^\mu\psi_j}^{j^\mu}  A_\mu  \\
            &\equiv -\frac{1}{4} F_{\mu\nu}F^{\mu\nu} + \sum_{j}\bar{\psi}_j(i\slashed{D}-m_j)\psi_j
\end{align}
with $q_j$ being the electric charge of the respective field, $\slashed{D} = \gamma^\mu D_\mu = \gamma^\mu (\partial_\mu + iqA_\mu)$ the covariant derivative and $A_\mu$ is the photon field and the index $j$ runs over all known elementary fermions:
\begin{align}
    \text{leptons: } &e,\,\mu,\,\tau,\,\nu_e,\,\nu_\mu,\,\nu_\tau\\
    \text{quarks: } &u,\,d,\,c,\,s,\,t,\,b
\end{align}
The Lagrangian in Eq.~(\ref{eq:L_QED}) is invariant under the gauge transformations:
\begin{align} \label{eq:QED_gauge_transformations} %Schwartz page 481
    \psi_j &\rightarrow \psi'_j = e^{iq_j\alpha(x)}\psi_j \\
    A_\mu &\rightarrow A_\mu' = A_\mu + \frac{1}{q} \partial_\mu \alpha(x)
\end{align}
and the associated motion equations are given by:
\begin{align}
    (i\slashed{D}-m_j)&\psi_j =0,\qquad \partial_\mu F^{\mu\nu}=j^\nu \\
    &\text{with: } k^\mu j_\mu = 0 \label{eq:Ward_idendity}
\end{align}
with the \textit{Ward identity} Eq.~(\ref{eq:Ward_idendity}) being equivalent to the current conservation Eq.~(\ref{eq:current_conservation}) in classical electrodynamics.

\myparagraph{Propagators} The propagator of a relativistic spin-$1/2$ particle equivalent to Eq.~(\ref{eq:QM_propagator}) could be derived by finding the Green's function of the Dirac operator Eq.~(\ref{eq:QMv1-Dirac-equation}):
\begin{alignat}{2}
(i\slashed{\partial}-m)S_F(x-y)&=iI_4\delta^4(x-y) \qquad &&\text{space-time representation} \\
(\slashed{p}-m)\tilde{S}_F(p)&=iI_4 \qquad &&\text{momentum representation}
\end{alignat} 
which leads to the following solutions:
\begin{alignat}{2}
    S_F(x-y)&=\int \frac{d^4p}{(2\pi)^4} e^{-ip(x-y)}S_F(p) \equiv \bra{0}T\psi(x)\bar{\psi}(y)\ket{0} \\
    \tilde{S}_F(p)&=\frac{(\slashed{p}+m)}{p^2-m_e^2+i\epsilon} \equiv \frac{1}{\slashed{p}-m+i\epsilon} \label{eq:fermion_propagator}
\end{alignat} 
where $i\epsilon$ is used as a prescription for integration in the complex plane, uniquely fixing the contour over which the integration is performed to obtain the Green's function~\cite{peskin2018introduction}. $T$ is for time-ordering allowing to sort out both cases where $x^0>y^0$ or $x^0<y^0$.
%and can be generally defined as:
%\begin{equation}
%    T\{A(x)B(y)\equiv \theta(t_x - t_y)A(x)B(y)\pm\theta(t_y-t_x)B(y)A(x)
%\end{equation}
%with $\theta$ denoting the Heaviside step function and the $\pm$ depends on %if the operators are bosonic ($+$) or fermionic ($-$).

Similarly, the photon propagator in Lorentz gauge is given by:
\begin{align}
    D(x-y)&=\bra{0}TA_\mu(x)A_\nu(y)\ket{0} = \int \frac{d^4k}{(2\pi)^4}\frac{-ig_{\mu\nu}}{k^2+i\epsilon}e^{-ik(x-y)}\\
    \tilde{D}(p)&= \frac{-ig_{\mu\nu}}{k^2+i\epsilon} \label{eq:photon_propagator}
\end{align}

\myparagraph{Perturbation theory and Feynman rules} Our final goal is to compute scattering cross sections in order to probe and analyse the hadronic structure in Chapter~\ref{chap:1}. The cross section is formally defined as:
\begin{equation}
\sigma = \frac{N}{\rho_A\cdot l_A\cdot\rho_B l_B\cdot A}    
\end{equation}
where $N$ is the number of scattering events, $A$ and $B$ are two colliding particle bunches having densities $\rho_A$ and $\rho_B$ and length $l_A$ and $l_B$ with A as the common area.
The probability that the initial state $\ket{\psi_A\psi_B}_{in}$ evolves into the final state $_{out}\bra{\psi_1\psi_2\dddot{}}$ is given by:
\begin{align}
    P &= |_{out}\braket{\psi_1\psi_2\dddot{}|\psi_A\psi_B}_{in}|^2\\
    _{out}\braket{\psi_1\psi_2\dddot{}|\psi_A\psi_B}_{in}  &=\lim_{T\rightarrow\infty}\braket{\bm{p}_1\bm{p}_2\dddot{}|e^{-iH(2T)}|\bm{k}_A\bm{k}_B} \\ &\equiv \braket{\bm{p}_1\bm{p}_2\dddot{}|S|\bm{k}_A\bm{k}_B} =\braket{\bm{p}_1\bm{p}_2\dddot{}|(\bm{1}+iT)|\bm{k}_A\bm{k}_B}
\end{align}
where the $S$-matrix or \textit{scattering matrix}~\cite{PhysRev.52.1107} encapsulates the scattering process of the initial and final states. When there's no interaction, $S=\bm{1}$ and therefore all the non-trivial scattering is captured by the T-matrix that we can express as follows:
\begin{align}
    \braket{\bm{p}_1\bm{p}_2\dddot{}|iT|\bm{k}_A\bm{k}_B} &\equiv (2\pi)^4\delta^{(4)}(k_Ak_b-\sum_fp_f)i\mathcal{M}(k_A,k_b\rightarrow p_f) \label{eq:T_matrix}\\
    &\implies d\sigma \propto |\mathcal{M}(k_A,k_B\rightarrow p_f)|^2
    \label{eq:cross_section}
\end{align}
with the $\delta^{(4)}$ function ensures momentum conservation. Unfortunately, we cannot solve analytically Eq.~(\ref{eq:cross_section}), i.e the interacting field theory as we did for the free theories. For that reason, we use perturbative expansion to derive the interaction term $H_{int}$ in terms of the coupling constant\footnote{Coupling constant: the couplings are not really constant, in QED the coupling becomes large at short distance and in QCD the opposite (asymptotic freedom).} (the fine structure constant $\alpha$ in QED). This approximation is valid and approaches the exact answer as long as the coupling is small enough to justify it.

This expansion can be represented diagrammatically as a sum of \textit{Feynman diagrams}~\cite{feynman1949theory}, a tool developed by Feynman 
%by means of \textit{Wick's theorem} that reduces the products of creation and annihilation operators to sums of products of their pairs. 
which allows to express the $S$-matrix up to any order of the perturbative expansion in terms of propagators and Dirac solutions. In case of QED the summary of Feynman rules reads:
%%! https://www.desy.de/~jlouis/Vorlesungen/QFTI10/QFTI.pdf

\begin{table}[!h] 
    \centering
    
    \begin{tabular}{ccccc}
  \toprule
        & Propagators & Incoming & Outgoing & Vertex \\
  \midrule
    Photon & $\tilde{D}(p)$ in Eq.~(\ref{eq:photon_propagator}) & $\epsilon_\mu^r(k)$ & $\epsilon_\mu^{\dagger r}(k)$ & \multirow{3}{*}{$-iq\gamma^\mu$}\\
    Fermion & \multirow{2}{*}{$\tilde{S}_F(p)$ in Eq.~(\ref{eq:fermion_propagator})}  & $u^s(p)$ & $\bar{u}^s(p)$ & \\
    Anti-fermion & & $\bar{v}^s(p)$ & $v^s(p)$ & \\
  \bottomrule
\end{tabular}
\caption{\small The QED Feynman rules. \label{tab:QEDFeynmanRules}}
\end{table}

\section{Group theory}
\label{app:group_theory}
The entirety of this appendix relies on \cite{Georgi:1999wka} and contains the main definitions and notions in group theory needed to construct our gauge theories. 

\subsection*{Definitions} 

\myparagraph{Group} A group $G$ is a set with a rule for assigning to every ordered pair of elements, a third element satisfying:
\begin{enumerate}
    \item if $f,g \in G$ then $h=fg \in G$.
    \item For $f,g,h \in G$, $f(gh)=(fg)h$.
    \item There's an identity element $e$ such that for all $f \in G, ef=fe=f$.
    \item Every element $f\in G$ has an inverse $f^{-1}$ such that $ff^{-1}=f^{-1}f=e$.
\end{enumerate}
An \textit{Abelian} group is one in which the multiplication law is commutative $g1g2=g2g1$.

\myparagraph{Representation} \label{s3:representation} A representation of $G$ is a mapping $D$ of the elements of $G$ onto a set of linear operators with the following properties:
\begin{enumerate}
    \item $D(e) = 1$, where $1$ is the identity operator in the space on which the linear operators act.
    \item $D(g_1)D(g_2)=D(g_1g_2)$, \textit{i.e} the group multiplication law is mapped onto the natural multiplication in the linear space on which the linear operators act.
\end{enumerate}

Some properties of representations:
\begin{itemize}
    \item As long as a transformation $S$ is invertible, one can always define a new representation $D'$ such that:
    \begin{equation}
        D(g) \rightarrow D'(g) = S^{-1}D(g)S
    \end{equation}
    where $D'$ is an \textit{equivalent} representation of $D$ differing only by the choice of basis.
    \item \textit{Unitary} representations are such that all operators $D(g)\dagger = D(g)^{-1} \quad [\forall g \in G]$.
    \item A representation is \textit{completely reducible} if it is equivalent to a representation whose matrix elements are in block diagonal form.
    \item Every representation of a finite group is equivalent to a unitary representation.
\end{itemize}

\subsection*{Lie groups}
We are mainly interested in continuously generated groups in the context of quantum field theory. Suppose our group elements $g \in G$ depend \textit{smoothly}\footnote{Smooth: If two elements of a group are "close" in the space of the group elements, so are the parameters that describe them.} on a set of continuous parameters $g(\alpha)$.

\myparagraph{Generators}
It is useful to parameterize the elements $g$ of the group $G$ that they're close to the identity element of the group, and such that $\alpha =0$ corresponds to the identity element $g(\alpha=0)=e$. We can therefore Taylor expand any representation $D(\alpha)$ in terms of the infinitesimal $d\alpha$ as:
\begin{equation} \label{eq:generators}
    D(d\alpha) = 1 + id\alpha_aX_a
\end{equation}
where $X_a=-i\partial_{\alpha_a}D(\alpha)$ for $a=1,...,N$ are the \textit{generators of the group}. There is enormous freedom to parameterise the group elements, we chose one by simply raising eq.~(\ref{eq:generators}) to some large power:
\begin{equation}
    D(\alpha)=\lim_{k\rightarrow\infty}(1 + id\alpha_aX_a)^k = e^{i\alpha_aX_a}
\end{equation}
which defines a particular \textit{exponential parameterization} of the representations.

\myparagraph{Lie algebra} 
Let $U(\lambda) = D(\alpha)^\lambda= e^{i\lambda\alpha_aX_a}$ the representation of a Lie group $G$. The multiplication law (See Section.~\ref{s3:representation}) is simply:
\begin{equation}
    U(\lambda_1)U(\lambda_2) = U(\lambda_1+\lambda_2)
\end{equation}
However if we multiply group elements generated by two different linear combinations of generators $X_a$ and $X_b$, in general:
\begin{equation}
    e^{i\alpha_aX_a}e^{i\beta_bX_b} \neq e^{i(\alpha_a+\beta_a)X_a}
\end{equation}
But since the exponentials form a representation of the group, we have to find a $\delta$ such as:
\begin{equation}
    e^{i\alpha_aX_a}e^{i\beta_bX_b} = e^{i\delta_aX_a}
\end{equation}
Interestingly, by Taylor expanding both sides, we can write:
\begin{align}
    i\delta_aX_a = i\alpha_aX_a + i\beta_aXa - \frac{1}{2}[\alpha_aX_a,\beta_bX_b]+\dddot{}
\end{align}
which we obtained only using the group property and smoothness. We conclude that:
\begin{equation}
    [\alpha_aX_a,\beta_bX_b]=-2i(\delta_c - \alpha_c - \beta_c)X_c+\dddot{} \equiv \gamma_cX_c
\end{equation}
Since the equality above must be true $\forall \alpha, \beta$, we must have $\gamma_c = \alpha_a\beta_bf_{abc}$ for some constants $f_{abc}$ and thus:
\begin{equation}
    [X_a,X_b]=if_{abc}X_c, \qquad f_{abc}=-f_{bac}
    \label{eq:Lie_algebra}
\end{equation}
We finally deduce the following properties of the Lie algebra:
\begin{itemize}
    \item The commutator in Lie algebra plays a role similar to the multiplication law for the group therefore it is enough to define the group.
    \item $f_{abc}$ are called the \textit{structure constants} of the group and the summarize the entire group multiplication law.
    \item eq.~(\ref{eq:Lie_algebra}) is called \text{Lie algebra} of the group which is completely determined by $f_{abc}$.
    \item A unitary representation of the algebra, requires that $f_{abc}$ are real.
    \item The matrix generators satisfy: $[X_a,[X_b,X_c]]+\text{cyclic permutations}=0$ called the Jacobi identity.
    \item The \textit{compact} Lie algebra is the special case where $f_{abc}$ is completely antisymmetric.
\end{itemize}

\myparagraph{SU(2)} \label{s3:SU2} The SU(2) algebra is defined by:
\begin{equation}
    [J_i,J_j]=i\epsilon_{ijk}J_k
    \label{eq:SU2_algebra}
\end{equation}
which is the simplest of the compact Lie algebras because $\epsilon_{ijk}$ is the simplest possible completely antisymmetric object with three indices.

The spin $1/2$ representation in terms of Pauli matrices:
\begin{align}
    J_1^{1/2} &= \frac{1}{2}\begin{pmatrix}
        0 & 1 \\ 1 & 0
    \end{pmatrix}
    = \frac{1}{2}\sigma_1 \\
    J_2^{1/2} &= \frac{1}{2}\begin{pmatrix}
        0 & -i \\ i & 0
    \end{pmatrix}
    = \frac{1}{2}\sigma_2\\
    J_3^{1/2} &= \frac{1}{2}\begin{pmatrix}
        1 & 0 \\ 0 & -1
    \end{pmatrix}
    = \frac{1}{2}\sigma_3
    \label{eq:Pauli}
\end{align}
is the simplest representation of SU(2), satisfying $\sigma_a\sigma_b=\delta_{ab}+i\epsilon_{abc}\sigma_c$ and given by the representation $e^{i\bm{\alpha}\cdot \bm{\sigma}/2}$ which makes it responsible for the name \textit{Special Unitary} as it has a determinant of $1$. All the other representations can be constructed by following a systematic procedure.

\myparagraph{SU(3)} SU(3) is the group of $(3\times 3)$ unitary matrices with determinant 1. It is generated by $t^a = \frac{1}{2}\lambda^a$ where $\lambda^a$ are the hermitian, traceless Gell-Mann matrices (considered as the standard basis):
\begin{align}
    \lambda_{1}&={\begin{pmatrix}0&1&0\\1&0&0\\0&0&0\end{pmatrix}} \quad
    \lambda_{2}={\begin{pmatrix}0&-i&0\\i&0&0\\0&0&0\end{pmatrix}} \quad
    \lambda_{3}={\begin{pmatrix}1&0&0\\0&-1&0\\0&0&0\end{pmatrix}} \quad\\
    \lambda_{4}&={\begin{pmatrix}0&0&1\\0&0&0\\1&0&0\end{pmatrix}} \quad
    \lambda_{5}={\begin{pmatrix}0&0&-i\\0&0&0\\i&0&0\end{pmatrix}} \quad
    \lambda_{6}={\begin{pmatrix}0&0&0\\0&0&1\\0&1&0\end{pmatrix}} \quad\\
    \lambda_{7}&={\begin{pmatrix}0&0&0\\0&0&-i\\0&i&0\end{pmatrix}} \quad
    {\displaystyle \lambda_{8}={\frac {1}{\sqrt {3}}}{\begin{pmatrix}1&0&0\\0&1&0\\0&0&-2\end{pmatrix}}.}
    \label{eq:Gell-Mann}
\end{align}
which are generalisations of the Pauli matrices as the first three Gell-Mann matrices contain the latter.

The generators obey the following relations:
\begin{align}
[t^a,t^b]&=if^{abc}t^c \\
Tr\{t^a t^b\} &= T_R \delta^{ab} \\
\sum_a t^a_{ij}t^a{jk} &= C_F \delta_{ik} \\
\sum_{c,d} f^{acd}f^{bcd} &= C_A \delta_{ab} \\
t^a_{ij}t^a_{kl} = T_R (\delta_{kl}\delta_{il}-\frac{1}{N_C}\delta_{ij}\delta_{kl})
\end{align}
where $f^{abc}$ is a totally antisymmetric structure constant of the group and $T_R=\frac{1}{2}$, $C_F=\frac{4}{3}$, $C_A=N_C=3$ are called the Casimirs of SU(3).

\subsection*{Unitary representation of the Galilean group} \label{s2:Galilean_group} 
%https://arxiv.org/pdf/2004.08661.pdf
The quantum non-relativistic particle is a unitary representation (See Appendix.~\ref{app:group_theory}) of the Galilean group, as much as a relativistic one (Section.~\ref{s3:Coupling_to_matter}) is a representation of the Lorentz group. We derive in the following very briefly the Galilean group and use it to show that the intrinsic spin, for instance, is not a specifically relativistic effect \cite{LevyLeblond:1967zz} in Section.~\ref{s3:Canonical_quantisation_EM}.

The Hilbert space formalism of quantum mechanics leads naturally to a study of the unitary representations of the Galilei group, therefore the matrix representation of the Galilean transformation $\mathcal{U}(\bm{R},\bm{\dot{\epsilon}},\bm{a},b)$ is given by:

\vspace{-15pt}\begin{minipage}{0.25\textwidth}
    \begin{equation*}
        \mathcal{U}=
        \begin{pmatrix}
            \bm{R} & \bm{\dot{\epsilon}} & \bm{a} \\
            0 & 1 & b \\
            0 & 0 & 1  
        \end{pmatrix}
    \end{equation*}
\end{minipage}
\begin{minipage}{0.7\textwidth}
\begin{alignat}{3}
    \text{Tran}&\text{sformations}  \qquad \text{Unitary}&&\text{ Operator} \nonumber\\%&&\qquad \text{ } \nonumber \\
    \bm{x} &\rightarrow R_i(\theta_i)\bm{x} \qquad &&e^{-i\theta_i \hat{J}^i} \\%&&\qquad \text{Rotations}\\
    \bm{x} &\rightarrow \bm{x} + \bm{a} \qquad &&e^{-i a_i \hat{P}^i} \\%&&\qquad \text{Space translations}\\
    \bm{x} &\rightarrow \bm{x} + \bm{\dot{\epsilon}}t \qquad &&e^{i \epsilon_i \hat{G}^i} \\%&&\qquad \text{Boosts}\\
    t &\rightarrow t + b \qquad &&e^{i b \hat{H}} %&&\qquad \text{Time translations}\\
\end{alignat}
\end{minipage}

where $\bm{R}$ is the ($3\times3$) rotation matrix, $\dot{\epsilon}$ and $a$ are the three-vectors of velocities and space-constants, $b$ is a time-constant. We notice that:
\begin{itemize}
    \item Setting $\bm{R}=I_3$, $\bm{a}=\bm{0}$ and $b=0$ reproduces the special case of uniform motion transformations in eq.~(\ref{eq:galilean_transformations}), denoted $(\bm{R}^3,+)$.
    \item Setting $\bm{v}=\bm{0}$, $\bm{a}=\bm{0}$ and $b=0$ lead to the rotation group SO(3).
\end{itemize}
% https://en.wikipedia.org/wiki/Galilei-covariant_tensor_formulation
% https://en.wikipedia.org/wiki/Galilean_transformation

the Galilean transformation $\mathcal{U}$ is represented by a set of four generators, $\hat{H}$ the generator of time translations (Hamiltonian operator), $\hat{\bm{P}}$ the generator of translations (momentum operator), $\hat{\bm{G}}$ is the generator of Galilean transformations (Boosts) and $\hat{\bm{J}}$ generator of rotations (angular momentum operator). The Lie algebra is represented by the following commutation relations:
\begin{align}
    &[\hat{H},\hat{P}_i] = [\hat{P}_i,\hat{P}_j] = [\hat{J}_{ij},\hat{H}] = [\hat{G}_i, \hat{G}_j] = 0\\
    &[\hat{J}_{i},\hat{J}_{j}] = i\hbar\epsilon_{ijk}\hat{J}_k; \qquad [J_{i},P_j]  = i\hbar\epsilon_{ijk} P_k; \qquad [J_{i},G_k] = i\hbar\epsilon_{ijk} \hat{G}_k \\
    &[\hat{G}_i, \hat{H}] = i\hbar \hat{P}_i; \qquad [\hat{G}_i,\hat{P}_j] = i\hbar M\delta_{ij}
\end{align}

The dual Galilean metrics are the time metric $t_{\mu\nu}=diag(1,0,0,0)$ and space metric $h_{\mu\nu}=diag(0,1,1,1)$ that satisfies the orthogonality condition $h^{\mu\nu}t_{\mu\nu}=0$, and by which $x_\mu x_\nu t^{\mu\nu}=t^2$ and $x_\mu x_\nu h^{\mu\nu}=|\bm{x}|^2$ are invariant.

\subsection*{Representation theory of the Lorentz group} \label{s2:Lorentz_group}
%http://physics.unm.edu/Courses/Finley/p581/Handouts/CompleteLorentzGroup.pdf
Similar to Section.~(\ref{s2:Galilean_group}), the Lorentz group denoted SO(1,3) (See Appendix.~\ref{app:group_theory}) expresses the invariance of the relativistic Lagrangian under Lorentz transformations $\Lambda_{\mu\nu}$ is represented by a set of six generators $J^{\mu\nu} = i(x^\mu \partial^\nu - x^\nu \partial^\mu)$ that consists of three rotations and three boosts in Minkowsi space such that $\Lambda^Tg\Lambda = g$ and with the associated unitary operator $e^{-iw_{\mu\nu}J^{\mu\nu}}$. 
The Lie algebra of the group is encapsulated in the following commutation relations:
\begin{align}
    [J^{\mu\nu},J^{\rho\sigma}] & =i(g^{\nu\rho}J^{\mu\sigma}-g^{\mu\rho}J^{\nu\sigma}-g^{\nu\sigma}J^{\mu\rho}+g^{\mu\sigma}J^{\nu\rho})
\end{align}

The Minkowsi metric is $g_{\mu\nu}=diag(1,-1,-1,-1)$ by which $x_\mu x_\nu g^{\mu\nu}=t^2 - |\bm{x}|^2$ is invariant.

At this stage, it is very useful to know that the $\Lambda$ matrices satisfies the Clifford algebra of some matrices $\gamma^\mu$ given by:
\begin{equation} \label{eq:Clifford_algebra}
\{\gamma^\mu,\gamma^\nu\}=2\eta^{\mu\nu} \implies \gamma^{'\mu}=\Lambda^{\mu\nu}\gamma_\nu = S^{-1}\gamma^\mu S \implies S^{\mu\nu}=\frac{i}{4}[\gamma^\mu,\gamma^\nu]
\end{equation}
when $\eta^{\mu\nu} = g^{\mu\nu}$ and where $\{A,B\} = AB + BA$ denotes the anti-commutation relation and $S$ is an invertible transformation that is determined by matching the infinitesimal transformation of $\Lambda = \delta - \frac{i}{2}w_{\mu\nu}J^{\mu\nu}$.
